# Supplementary material for: Controlling Character Motions without Observable Driving Source
Source: arXiv:2308.06025 source file (2023-08-11)
Supplement: Supplementary file 1 [file appendix.tex]

\section{Experiment Settings}
\subsection{VQ-VAE}
The encoder of VQ-VAE network is constructed by a fully-connected network with 3 hidden layers of [512, 512, 512] units, followed by a linear network to 64 dimension latent space. The decoder of VQ-VAE network is constructed by the same structure with the encoder. The output dimension of the decoder is the feature space of different dataset, which is 45 in Trinity Gesture datasets, 56 in VTuber-EMOCA datasets and 72 in AIST++ datasets.

We use the Adam optimizer with the initial learning rate being $1\times10^{-4}$. The learning rate is decayed by a factor of 0.96 every two epochs. 
% The batch size for Trinity dataset is 1000 while that for VTuber-EMOCA dataset is 20000. 
The batch size for different datasets varies, with Trinity dataset having a batch size of 1000, VTuber-EMOCA dataset having a batch size of 20000, and AIST++ having a batch size of 256.
All the models are trained for 200 epochs, which takes about half an hour on a single NVIDIA V100 GPU.

\subsection{Low-Level Policy}
The low-level policy network is constructed by a fully-connected network with 3 hidden layers of [1024, 1024, 512] units, followed by linear output units. The value function is modeled by a similar network, but with a single linear output unit. The encoder and discriminator are jointly modeled by a single network but with separate output units.
We used Tanh activations for hidden layers in PPO algorithms while ReLU activations are used for the other hidden units.

During training, the task tokens are randomly sampled from the activated code in the codebook pre-trained in the high-level policy. 256 environments are simulated in parallel on a single NVIDIA V100. The low-level policy is trained with over 6 billion samples, requiring about 2 days on a single GPU.    %% 200k * 256 * 128
% \subsection{Hyperparameters}

The detailed hyperparameter settings used in low-level policy are available in Table \ref{low-level hyper}.
%, and the hyperparameters for prior high-level policy are avaliable in Table \ref{high-level hyper}.
% Details of the low-level policy network.
\begin{table}[!ht]
    \centering
    \begin{tabular}{|l|c|}
    \hline
        \textbf{Parameter} & \textbf{Value} \\ \hline
        Token Embedding Dim & 64 \\ \hline
        Action Distribution Standard Deviation & 0.2 \\ \hline
        Window Size $\Delta T$ & 10 \\ \hline
        Realistic Reward Weight & 2 \\ \hline
        Diversity Reward Weight & 0.2 \\ \hline
        Correspondence Reward Weight & 0.5 \\ \hline
        Discriminator/Encoder Minibatch Size & 4096 \\ \hline
        Policy/Value Function Minibatch Size & 4096 \\ \hline
        Adam Stepsize & 1e-5 \\ \hline
        $\gamma$ Discount & 0.98 \\ \hline
        TD$(\lambda)$ & 0.95 \\ \hline
        GAE$(\lambda)$ & 0.95 \\ \hline
        PPO Clip Threshold & 0.2 \\ \hline
        $T$ Episode Length & 128 \\ \hline
    \end{tabular}
    \caption{Hyperparameters for training low-level policy.}
    \label{low-level hyper}
\end{table}

\subsection{High-Level Policy}
For the autoregressive high-level policy, we use a $4$-layer transformer with 8 heads. The embedding size is $512$ while the hidden size is $256$. The training scheme is the same as that of the VQ-VAE model, which takes about $4$ hours on a single NVIDIA V100 GPU.

During the inference period, the prior tokens are generated in an autoregressive pattern with past token length of 20. We adopt the top-$k$ sampling strategy to add some randomness with $k$ being $5$. We also add a temperature ($=10$) when calculating the probability distribution over the selected $k$ tokens using softmax.

For the random high-level policy, there is no need to build a model and train it. We only need to randomly sample from the codebook every 20 frames. Interestingly, this scheme achieves surprisingly good results, even better than all the other methods on Trinity dataset.

\subsection{User Study}
Besides, we apply user study on the Trinity dataset to further evaluate the sequence quality of different algorithms. For each algorithm, we generate twenty 10-second clips. Five independent users are invited to rate the clips with score ranging from 1 to 5. $10$ ground-truth clips are first represented before rating. Then we obtain $20\times5$ scores for each algorithm. The average score with error bar is shown in Fig.~\ref{fig:user_study}. Our algorithm achieves the best performance (4.73) while the score of the second best method ASE is 1 point lower (3.73).

\begin{figure}[t]
    \centering
    \includegraphics[width=0.8\linewidth]{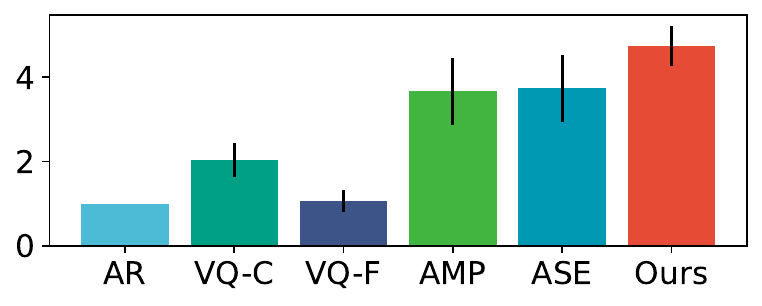}
    \caption{Average score of different algorithms annotated by 5 independent users. Our algorithm produces the highest score among all the comparing methods.}
    \label{fig:user_study}
\end{figure}
